# Supplementary material for: Entanglement Distillation between Solid-State Quantum Network Nodes
Source: arXiv:1703.03244 ancillary file (2017-03-09)
Supplement: Supplementary file 1 [file SupplementalMaterial.pdf]

# Supplementary Information

## Entanglement Distillation between Solid-State Quantum Network Nodes

N. Kalb,<sup>1,2,\*</sup> A. A. Reiserer,<sup>1,2,†</sup> P. C. Humphreys,<sup>1,2,\*</sup> J. J. W. Bakermans,<sup>1,2</sup> S. J. Kamberling,<sup>1,2</sup>

N. H. Nickerson,<sup>3</sup> S. C. Benjamin,<sup>4</sup> D. J. Twitchen,<sup>5</sup> M. Markham,<sup>5</sup> and R. Hanson<sup>1,2,‡</sup>

<sup>1</sup>*QuTech, Delft University of Technology, P. O. Box 5046, 2600 GA Delft, The Netherlands*

<sup>2</sup>*Kavli Institute of Nanoscience, Delft University of Technology,  
P. O. Box 5046, 2600 GA Delft, The Netherlands*

<sup>3</sup>*Department of Physics, Imperial College London, Prince Consort Road, London SW7 2AZ, U.K.*

<sup>4</sup>*Department of Materials, University of Oxford, Parks Road, Oxford OX1 3PH, U.K.*

<sup>5</sup>*Element Six Innovation, Fermi Avenue, Harwell Oxford, Didcot, Oxfordshire OX11 0QE, U.K.*

### I. EXPERIMENTAL DESIGN

We use chemical-vapour-deposition homoepitaxially grown diamonds of type IIa with a natural abundance of carbon isotopes. Both diamonds have been cut along the  $\langle 111 \rangle$  crystal axis and were grown by Element Six. They are situated in home-built confocal microscope setups within closed-cycle cryostats (4 K, Montana Instruments) separated by two meters. We additionally employ a magnetic field (Node A: 418.248(5) G; node B: 413.980(5) G) approximately aligned with the NV symmetry axis in both setups by placing a permanent magnet within the respective sample chamber and compensating slight alignment-deviations with additional permanent magnets from the outside (few cm distance). Microwave pulses are applied via a gold stripline (thickness of 200 nm) that has been deposited onto the surface of the sample. We shape these pulses to a Hermite amplitude envelope for robustness against qubit frequency detunings ( $\approx$  MHz) such as arising from the hyperfine interaction with the host nitrogen nuclear spin [1]. To generate short optical excitation pulses, we use an electro-optic modulator (Jenoptik) in a homebuilt, temperature stabilized, enclosure which, in conjunction with an upstream acousto-optic modulator (Gooche & Housego), creates a laser pulse with high on/off ratio and Gaussian temporal envelope. This pulse is split into two using a polarization maintaining fiber beam splitter (Evanescence Optics) for excitation of both NV centers. Optical transition frequencies of each NV center are tuned by applying voltages to gold electrodes on the diamond surface (see also Section V).

We employ a single-layer anti-reflection coating for 637 nm light ( $\text{Al}_2\text{O}_3$ ) and solid immersion lenses around the position of the NVs to increase optical collection efficiencies. This in conjunction with the cryogenic environment allows for spin-selective optical read-out of the NV electron spin in a single-shot via the optical

$E_x$  ( $E_y$ ) transition on node A (node B). We measure read-out fidelities of 0.9379(6) (0.8985(7)) for the bright  $|m_s = 0\rangle \equiv |0\rangle$  ground-state and 0.9932(2) (0.9962(1)) for the dark  $|m_s = +1\rangle \equiv |1\rangle_A$  ( $|m_s = -1\rangle \equiv |1\rangle_B$ ) state on node A (node B). These values are subsequently used to correct for read-out errors of the electron spins in state tomography measurements. Node A additionally uses adaptive optics to compensate for imperfections in the solid immersion lens, which leads to an improved collection efficiency of zero-phonon-line (ZPL) photons [1].

We utilize each electron spin to control an adjacent nuclear spin ( $I = \frac{1}{2}$ ) associated with a  $^{13}\text{C}$  atom in the diamond lattice via dynamical decoupling sequences that are resonant with the electron-nuclear dynamics, optimizing the gate parameters to maximize the fidelity of our operations. The parameters for a full entangling operation between nuclear and electron spin are given in Table S1. Furthermore we characterize the strength of the magnetic hyperfine interaction between nuclear spin and electron as well as nuclear dephasing times with the electron spin idling in one of the two relevant states ( $|0\rangle$  or  $|1\rangle$ ). The decay of the memories when performing entangling attempts are best fit with exponential functions of the form  $e^{-(t/T)^n}$  with  $T$  the  $1/e$  decay constant and with exponents  $n = 1.7(1), 1.48(5)$  for nodes A and B respectively. We correct for tomography errors on the nuclear spin state by employing previously developed methods that rely on a symmetric initialization and read-out of the respective nuclear spin [2, 3]. The measured quantities are given in Table S1.

### II. EXPERIMENTAL SEQUENCE

Remote entangled electron spin states are generated by initializing the superposition state  $|\theta\rangle$  on both sides (we use a  $2\mu\text{s}$  long repumping laser pulse followed by a microwave pulse) and subsequent optical excitation from a common laser source which guarantees relative frequency-stability. The sequence duration is  $7\mu\text{s}$ . A photo-detection event heralds the desired raw state of Eq. (2). We obtain single-photon detection probabilities of  $p_a = 8 \cdot 10^{-4}$  ( $p_b = 4 \cdot 10^{-4}$ ) for node A (node B). A final microwave  $\pi$ -pulse preserves electron coherence and decouples the magnetic hyperfine interaction with

\* These authors contributed equally

† Present address: Max-Planck-Institute for Quantum Optics, Hans-Kopfermann-Str. 1, 85748 Garching, Germany

‡ To whom correspondence should be addressed; E-mail: [r.hanson@tudelft.nl](mailto:r.hanson@tudelft.nl)

|                       | Node A              | Node B             | Description                                                              |
|-----------------------|---------------------|--------------------|--------------------------------------------------------------------------|
| $A_{\parallel}$ (kHz) | $-2\pi \cdot 30(1)$ | $2\pi \cdot 33(1)$ | Parallel hyperfine coupling with electron spin.                          |
| $A_{\perp}$ (kHz)     | $2\pi \cdot 88(1)$  | $2\pi \cdot 35(1)$ | Perpendicular hyperfine coupling with electron spin.                     |
| $N$                   | 12                  | 34                 | Number of inversion pulses on electron for nuclear spin gate.            |
| $\tau$ ( $\mu$ s)     | 21.772              | 12.812             | Optimized interpulse delay for nuclear spin gate.                        |
| $F_{\text{tomo}}$     | 0.973(3)            | 0.978(2)           | Correction factor for gate errors in the tomography sequence.            |
| $T_{2,0}^*$ (ms)      | 3.4(1)              | 19.4(3)            | Nuclear dephasing time with the electron idle in $ m_s = 0\rangle$ .     |
| $T_{2,1}^*$ (ms)      | 3.4(1)              | 16.2(3)            | Nuclear dephasing time with the electron idle in $ m_s = \pm 1\rangle$ . |
| $\sigma$              | 273(5)              | 272(4)             | fitted $1/e$ value of the memory decay in entangling attempts.           |

TABLE S1. Measured experimental parameters of the nuclear spins

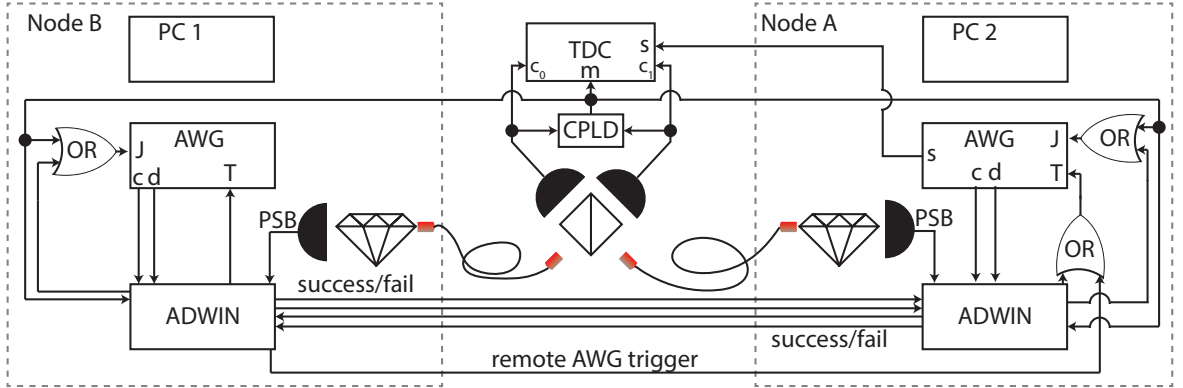

FIG. S1. Control schematic of the experimental setup. Complex programmable logic device (CPLD) outputs a trigger upon detection of a ZPL photon (see Section IV for timing). Time-to-digital converter (TDC, PicoQuant HydraHarp 400) with time-tagged channels ( $c_0$  and  $c_1$ ), a marker for ZPL photon detection events ( $m$ ), and a sync channel ( $s$ ). We use microprocessors for decision making (Jäger ADwin Pro II (ADwin)) and arbitrary waveform generators (Tektronix AWG5014c (AWG)) which have input channels for jump (J) and trigger (T) commands. Outputs of the AWGs are used to have the respective local ADwin count the number of entangling events ( $c$ ) and to determine whether a part of the logical sequence (see Fig. S2) has finished ( $d$ ). Besides, AWGs and ADwins control all laser and microwave pulses of the respective setup. Personal computers (PCs 1 & 2) are used for sequence programming, hardware control and monitoring during measurements. ADwins communicate success or failure of logical steps within the sequence with a three-way handshake that utilizes two digital input and two digital output channels on each device (success/fail). See Fig. S2 for further details on the sequence. The start of the AWG sequences is triggered via one ADwin to mitigate timing jitter between both AWG outputs.

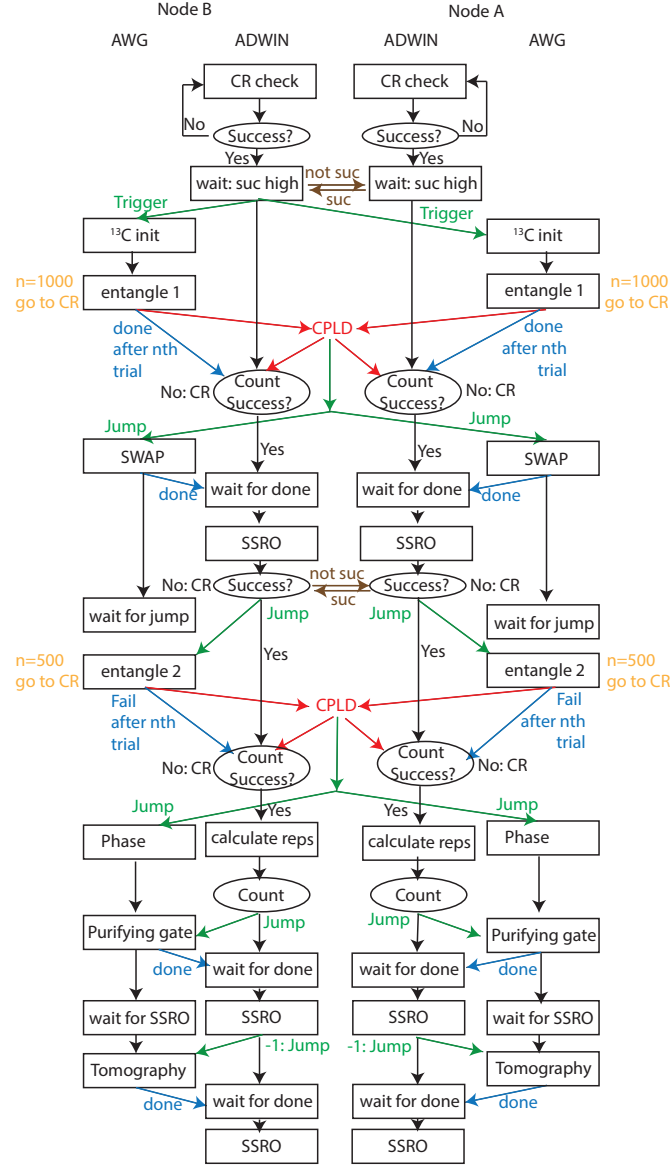

FIG. S2. Logical blocks for the AWG and ADWIN of each setup during one round of distillation. For a wire diagram of the experimental logic see Fig. S1. Boxes give logical steps within the sequence (see also Fig. 1C of the main text). Conditional actions and feedback are implied by ellipses. Before each experimental run we verify that both electron spins are on resonance via a charge-resonance (CR check) [4]. Unless indicated otherwise, black arrows represent an unconditional advance of the sequence even if no communication signal was received. The absence of a black arrow indicates a restart of the sequence upon failure.

the memory [5].

Generating remote entangled states with low detection efficiencies requires complex logic operations to limit overhead and guarantee a time-efficient execution of the sequence. We implement charge resonance checks for pre-selection of and feedback on the current NV emission frequencies as well as multiple logical stages in the sequence at which both nodes communicate local success or failure. Combined success events advance the sequence one step further whereas failure causes a restart. A schematic of the electrical wiring is depicted in Fig. S1. Fig. S2 gives an overview of all communication steps between all involved instruments.

### III. CONFIRMATION HERALD FOR A HIGH FIDELITY SWAP

The fidelity of the local swap operation is improved by constructing a confirmation herald. Prior to the swap the memory is initialized in the phase-insensitive eigenstate  $|0\rangle$  which gets mapped onto the fluorescing electron state  $|0\rangle$  by the applied gate sequence. Measuring the electron in the state  $|0\rangle$  by detection of a photon after the swap sequence therefore suppresses infidelities at negligible cost in efficiency (measured success probability of 0.89(1)).

### IV. TEMPORAL FILTERING & CPLD TIMING

We determine the relative timing of clicks originating from avalanche photodiodes (APDs) 1 and 2 by creating histograms of all detection events registered from each APD by the TDC. The maximum of the autocorrelation between these histograms indicates the timing delay at which the two temporal distributions are best overlapped.

Once this timing is determined, we fit a Gaussian profile to the beginning of the histogram of all overlapped data (Fig. S3). This Gaussian profile is known to closely correspond to our excitation pulse profile. We use this fit to estimate the point in time beyond which the ratio between photons from the excitation laser and the integrated residual NV emission is less than 0.001. This independently determined time set the beginning of the temporal filter in our analysis of the distillation results. We choose this conservative criterion in order to mitigate any potential impact of non-Gaussian tails in the laser profile.

In order to minimize the impact of dark counts, we set the end of the temporal filter to be 40 ns after the start of the window. This filtering is chosen because, for times longer than 40 ns after the excitation pulse, the ratio between dark counts and NV photon detections is estimated to increase above 0.1 for the most sensitive case ( $\theta = \pi/8$ ). A live temporal filter through the CPLD (see Figs. S1 and S2) allows us to exclude 36.6 % of all events on-the-fly.

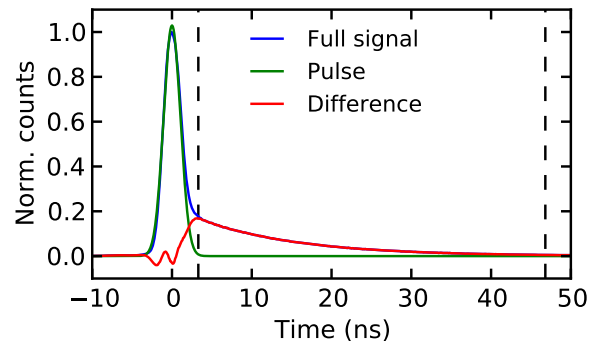

FIG. S3. Plotted in blue is the histogram of the timings of all APD clicks registered by our time-to-digital converter (blue). We fit a Gaussian profile to the beginning of this histogram (green), as this profile is known to closely correspond to the temporal shape of our excitation pulse. The profile of the NV emission (red) is estimated by taking the difference between the full histogram of counts and the photons assumed to originate from the excitation pulse. Dashed lines indicate the beginning and end of the detection window. Time is given with respect to the fitted center of the laser pulse.

### V. OPTICAL TRANSITION FREQUENCIES OF THE NV IN A MAGNETIC FIELD

Lateral crystal strain modifies the eigenstates and respective eigenenergies of the NV excited electronic states. Fig. S4 shows the optical transition frequencies  $\omega_{Ex}$  for  $|m_s = 0\rangle \rightarrow |E_x\rangle$  and  $\omega_{\pm 1}$  for the transitions  $|m_s = \pm 1\rangle \rightarrow |A_1\rangle$ , as a function of lateral strain. The transition  $|m_s = 0\rangle \rightarrow |E_x\rangle$  is of particular interest as it remains spin conserving even under large lateral strain fields (no deterioration was found for strain induced frequency shifts up to 5 GHz). Without magnetic field the ground states  $|m_s \pm 1\rangle$  are degenerate and  $\omega_{+1} = \omega_{-1}$ . In this case, at a lateral strain-induced frequency shift around 3.5 GHz  $\omega_{Ex}$  and  $\omega_{\pm 1}$  are nearly degenerate which hampers the quality of spin-photon entanglement. Applying a sufficiently large magnetic field along the NV axis splits the ground states due to the Zeeman effect; therefore  $\omega_{Ex}$  is degenerate with  $\omega_{+1}$  and  $\omega_{-1}$  in distinct strain regimes and there is always a choice of qubit states in the ground state triplet of the NV center that allows for high-quality spin-photon entanglement. In our experiment node A operates at a lateral strain-induced frequency shift of  $\sim 4$  GHz such that we choose  $|1\rangle \equiv |m_s = +1\rangle$ . These considerations are not a factor for node B, as in this case we are using the transition  $|m_s = 0\rangle \rightarrow |E_y\rangle$ .

### VI. DISTILLATION PROTOCOL

We entangle distant NV spins by employing single photons as flying qubits in a probabilistic measurement-

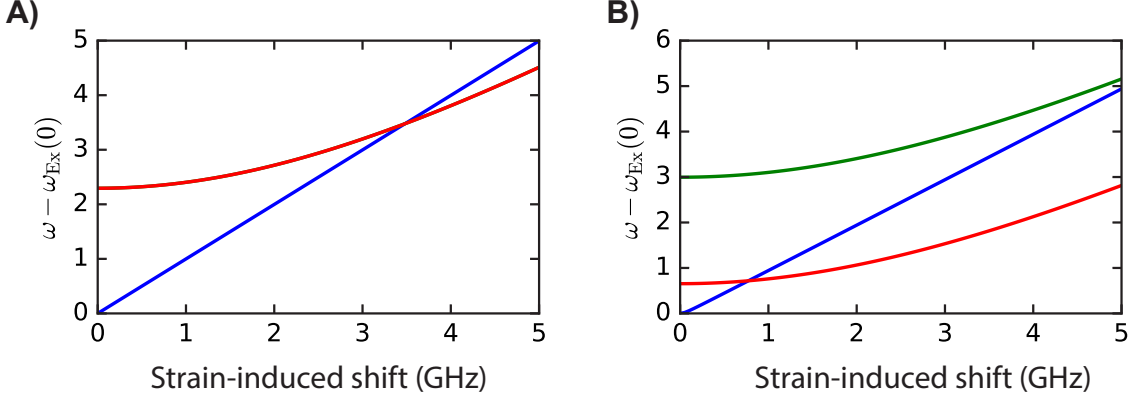

FIG. S4. Optical transition frequencies of the NV electron spin as a function of lateral strain with and without magnetic field. A) without magnetic field and B) with magnetic field along the NV axis ( $B = 418.2$  G). In the latter case the excitation frequencies  $\omega_{\pm 1}$  are no longer degenerate. Blue: transition from  $|m_s = 0\rangle$  to  $|E_x\rangle$ . Red (green): transition from  $|m_s = +1 (-1)\rangle$  to the optically excited state  $|A_1\rangle$ . Red and green lines overlap in panel A.

based entanglement (MBE) protocol. After initializing each NV in the  $|m_s = 0\rangle$  ground state, which we will label  $|0\rangle$ , a microwave pulse is used to rotate the spin into a superposition of this state and one of the  $|m_s = \pm 1\rangle$  states, here labeled  $|1\rangle$ . This prepares each NV in the state

$$|\theta\rangle = \sin \theta |0\rangle - i \cos \theta |1\rangle. \quad (1)$$

Subsequent spin-selective resonant excitation of the NVs leads to the emission of a single photon if the NV is in the  $|0\rangle$  state, creating spin-photon entangled states at each node. These single photons are transmitted to a central node and subsequently interfered on a beam splitter. In the ideal case, detection of a single photon after this beam splitter projects the NVs onto the entangled state  $|\Psi^\pm\rangle = -i(|01\rangle \pm |10\rangle)/\sqrt{2}$  (where the sign depends on which detector clicked).

We do not stabilize the phase of the excitation laser at the position of the NVs, nor the optical path length traversed by the emitted photons from the NVs to the central node. These differences between the two optical paths apply an unknown phase  $\phi$  to the entangled state. In addition, the NVs only emit photons 3% of the time in the usable zero-phonon line (ZPL), and the optical channels have finite transmissivities. This leads to a reduced

probability  $p_d$  of successfully detecting a single photon given that one of the NVs was in the  $|0\rangle$  state. These dominant imperfections mean that we actually produce the state

$$\rho_{\text{raw}}(\phi) = \eta |\Psi^\phi\rangle \langle \Psi^\phi| + (1 - \eta) |00\rangle \langle 00|, \quad (2)$$

where  $|\Psi^\phi\rangle = (|01\rangle + e^{i\phi} |10\rangle)/\sqrt{2}$  and  $\eta$  depends on both  $\theta$  and  $p_d$ .

Each communication qubit is flipped by applying  $R_x(\pi)$  as part of our dynamical decoupling sequence and then (following [6, 7]) swapped onto local memories at each node. This allows us to reuse the NVs to produce a second entangled state between the nodes. Upon success, our overall state is then given by  $\rho_{\text{raw}}(\phi_2) \otimes \rho'_{\text{raw}}(\phi_1)$ , where  $\phi_2$  and  $\phi_1$  depend on the phase differences at the two different times that the states were created (for pedagogical clarity, here we assume that the same detector clicked). Due to the particular swapping operation we employ, the memory state  $\rho'_{\text{raw}}(\phi_1)$  is a rotated version of the initial state  $\rho_{\text{raw}}(\phi_1)$ , such that  $\rho'_{\text{raw}}(\phi_1) = U \rho_{\text{raw}}(\phi_1) U^\dagger$ . Therefore, for readability, in the following text we redefine the memory qubit states in a rotated basis such that the states  $|0\rangle_m$  and  $|1\rangle_m$  are superpositions of the energy eigenstates  $|0\rangle$  and  $|1\rangle$  that are employed in the main text.

$$\begin{aligned} (|10\rangle_c + e^{i\phi_2} |01\rangle_c) \otimes (|10\rangle_m + e^{i\phi_1} |01\rangle_m) &\rightarrow (|11\rangle_c + e^{i\phi_2} |00\rangle_c) \otimes |10\rangle_m + e^{i\phi_1} (|00\rangle_c + e^{i\phi_2} |11\rangle_c) \otimes |01\rangle_m, \\ (|10\rangle_c + e^{i\phi_2} |01\rangle_c) \otimes |11\rangle_m &\rightarrow (|10\rangle_c + e^{i\phi_2} |01\rangle_c) \otimes |11\rangle_m, \\ |11\rangle_c \otimes (|10\rangle_m + e^{i\phi_1} |01\rangle_m) &\rightarrow |10\rangle_c \otimes |10\rangle_m + e^{i\phi_1} |01\rangle_c \otimes |01\rangle_m, \\ |11\rangle_c \otimes |11\rangle_m &\rightarrow |11\rangle_c \otimes |11\rangle_m \end{aligned} \quad (3)$$

Measurement of both communication qubits in the  $|00\rangle_c$  state heralds successful distillation. For a balanced superposition state ( $\theta = \pi/4$ ) and high photon loss ( $p_d \ll 1$ ), in which case  $\eta = 1/2$ , the distillation succeeds with probability  $\frac{1}{8}$ . It can be seen that this projects the memories into the pure state  $\frac{1}{\sqrt{2}}(e^{i\phi_1}|01\rangle_m \otimes e^{i\phi_2}|10\rangle_m)$ , and so the  $|11\rangle\langle 11|$  contamination has been removed.

In addition, if the phase drift over the duration of the experiment is sufficiently small, such that  $\phi_1 \approx \phi_2$ , one obtains the desired entangled state  $|\Psi^+\rangle = \frac{1}{\sqrt{2}}(|01\rangle_m + |10\rangle_m)$ . If different detectors clicked in the first and second rounds of entanglement generation, it can be easily shown that the resulting state is instead  $|\Psi^-\rangle = \frac{1}{\sqrt{2}}(|01\rangle_m - |10\rangle_m)$ .

In reality, our experiment has further experimental imperfections beyond optical phase drifts, and so the state that is actually produced by the distillation protocol deviates from this ideal entangled state. In our experiment, the primary imperfections are given in Table S2, along with independent estimates of their magnitudes. We incorporate these parameters into an analytical model of the experiment, as is outlined in the following section.

The independently estimated parameters are not sufficient to completely explain the obtained state fidelities. We therefore introduce two phenomenological parameters: an initial amplitude damping implemented via a dephasing operation ( $p = 0.08$ ) on the memory qubits and additional interferometric drift of the setup per entangling attempt. We fit our model to the combined dataset for all excitation angles. The resulting fit (3.4 mrad per entangling attempt) suggests an increased drift of the relative phase between both raw states which could be caused by a deviating interferometric stability at the time of data acquisition. In order to make a conservative comparison, these additional experimental infidelities are excluded for the modeled stored raw state that we compare with the purified state in Fig. 4B of the main text. Fig. S5 shows the state decay for all measured superposition angles and the result from fitting the model to the combined data set.

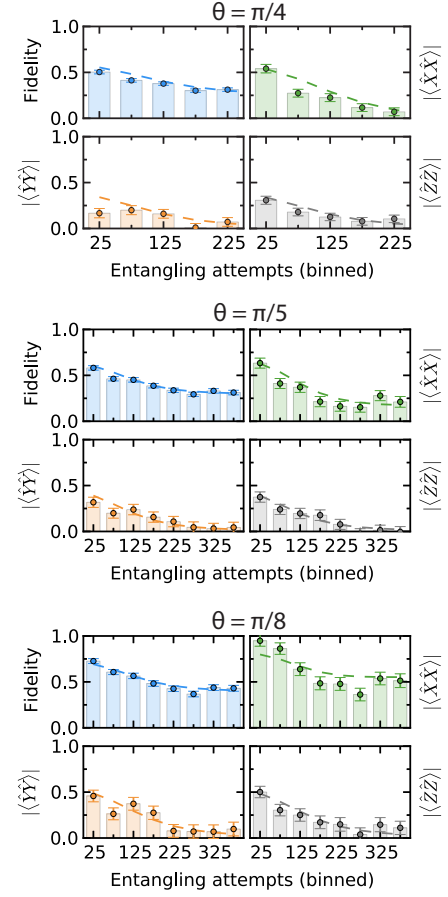

FIG. S5. Modeled (dashed lines) and measured correlations and state fidelities for all remaining excitation angles. See Fig. 4C of the main text for the data of  $\theta = \pi/6$ .

| Param.            | Value               | Description                                                                                                         |
|-------------------|---------------------|---------------------------------------------------------------------------------------------------------------------|
| $V$               | 0.72                | Indistinguishability between photons produced by the two NVs (Section VIII).                                        |
| $p_s$             | 0.01                | Failure probability for classical spin-photon correlations [1].                                                     |
| $p_{d1}$          | $8 \cdot 10^{-4}$   | Single-photon detection probability after the central beam splitter, given that NV <sub>1</sub> is in $ 0\rangle$ . |
| $p_{d2}$          | $4 \cdot 10^{-4}$   | Single-photon detection probability after the central beam splitter, given that NV <sub>2</sub> is in $ 0\rangle$ . |
| $p_{dc}$          | $2.5 \cdot 10^{-6}$ | Dark count probability within detection window.                                                                     |
| $p_{\text{gate}}$ | 0.0163              | Error rate for electron-nuclear-spin two-qubit gates.                                                               |
| $p_{\text{proj}}$ | 0.985               | Probability that the NV is left in $ m_s = 0\rangle$ , given the corresponding SSRO measurement result.             |
| $\phi$            |                     | First entangled state phase. The ideal protocol is insensitive to this parameter.                                   |
| $\Delta\phi$      | Section IX          | Difference in phase between the two entangled states.                                                               |
| $p_m$             | Sections I & VII B  | Memory dephasing probability during the interval between the generation of the two entangled states.                |

TABLE S2. Measured experimental parameters used in our error model.

## VII. EXPERIMENTAL MODEL

### A. Raw state

The raw entangled state in our model is given by

$$\rho_{\text{raw}} = p_{00} |00\rangle\langle 00| + p_{11} |11\rangle\langle 11| + |\Psi^\pm\rangle\langle \Psi^\pm| \quad (4)$$

where

$$|\Psi^\pm\rangle\langle \Psi^\pm| = \begin{pmatrix} \frac{1}{2}p_s(p_{01} + p_{10}) & 0 & 0 & 0 \\ 0 & p_{01}(1 - p_s) & \pm\sqrt{V p_{01} p_{10}}(1 - p_s)e^{i\phi} & 0 \\ 0 & \pm\sqrt{V p_{01} p_{10}}(1 - p_s)e^{-i\phi} & p_{10}(1 - p_s) & 0 \\ 0 & 0 & 0 & \frac{1}{2}p_s(p_{01} + p_{10}) \end{pmatrix}. \quad (5)$$

This state is parametrized by

$$\begin{aligned} p_{11} &= 2 \cos^4 \theta p_{\text{dc}} (1 - p_{\text{dc}}) \\ p_{10} &= \sin^2 \theta \cos^2 \theta ((1 - p_{\text{dc}})^2 p_{\text{d2}} + 2 p_{\text{dc}}(1 - p_{\text{dc}})(1 - p_{\text{d2}})) \\ p_{01} &= \sin^2 \theta \cos^2 \theta ((1 - p_{\text{dc}})^2 p_{\text{d1}} + 2 p_{\text{dc}}(1 - p_{\text{dc}})(1 - p_{\text{d1}})) \\ p_{00} &= \sin^4 \theta ((1 - p_{\text{dc}})^2 (p_{\text{d1}}(1 - p_{\text{d2}}) + p_{\text{d2}}(1 - p_{\text{d1}})) + 2(1 - p_{\text{dc}}) p_{\text{dc}}(1 - p_{\text{d1}})(1 - p_{\text{d2}})). \end{aligned} \quad (6)$$

### B. Protocol

We model the swap gate that transfers the entangled state to the nuclear spins at each node by assuming that this gate causes random two-qubit Pauli noise with a probability  $2 \times p_{\text{gate}}$ . As in the experiment, this swap gate stores the entangled state in a rotated basis, such that the initial electronic state is transformed by a Hadamard gate as it is stored.

After this swap, the stored state experiences dephasing noise due to the second round of entanglement attempts. This is modeled by applying a  $R_z(\pi)$  rotation independently to each of the stored states with a probability  $p_m$ . For Gaussian dephasing noise (such as decoherence), in which the fidelity of a stored state degrades as  $F = \frac{1}{2}(1 + e^{-\frac{n^2}{2\tau^2}})$ ,  $p_m = 1 - F \equiv \frac{1}{2}(1 - e^{-\frac{n^2}{2\tau^2}})$ . For exponential damping noise (such as the stochastic repumping process used to reset our NV spins [5]),  $p_m$  is given by  $\frac{1}{2}(1 - e^{-\frac{n}{\tau}})$ . Besides the induced dephasing due to the electron spin reset, we find that our feedback resolution is limited by systematic drifts of the required feedback phase per entangling attempt. Analyzing all calibration data results in an additional phase uncertainty of 0.87(3) mrad per entangling trial per node which is taken into account via a Gaussian decay channel.

We introduce a second raw entangled state, modeling the optical phase drift since the first state was generated by applying a  $R_z(\pi)$  rotation to one of the qubits with a probability determined by the expected phase drift  $\Delta\phi$  per attempt (Section IX).

The distillation operation consists of another two-qubit gate between the electron and the nuclear spin at each

node, and again is modeled by assuming random two-qubit Pauli noise, this time with a probability  $p_{\text{gate}}$ . Finally, we calculate the state of the nuclear spins after a noisy measurement of the electron spin, with a failure probability given by  $p_{\text{proj}}$ .

## VIII. TWO-PHOTON QUANTUM INTERFERENCE

We are able to estimate the degree of indistinguishability between the single photons emitted by each NV by aggregating the full set of detection events from the distillation data set. Using the same temporal filtering as for the distillation analysis, we calculate the number of events within this data set in which both APDs detect a photon within the same entanglement generation element. This is normalized by calculating the number of events in which one APD clicked in a given entanglement generation element, while the other APD clicked in the next entanglement generation element.

For fully distinguishable single-photon emission and balanced emission probabilities, the ratio  $r$  between coincident clicks to clicks in successive elements should be 0.5, while for fully indistinguishable photons no coincident clicks will be detected due to two-photon Hong-Ou-Mandel quantum interference [8]. This is because this quantum interference effect ensures that the two photons will always emerge from the same port of the beam splitter, and so both APDs will never click during the same round. For partially indistinguishable photons and again assuming balanced emission probabilities,  $r$  is related to the wave function overlap  $V = |\langle \psi_a | \psi_b \rangle|^2$  by

$V = (1 - 2r)$ . Incorporating the effect of the known imbalance in emission probabilities in our experiment, we find  $V = 0.72(3)$ . This is substantially lower than measured in Refs. [1, 9]. We hypothesize that this is due to fast spectral diffusion of one of our NVs, which is not picked up by our charge resonance checks as they confirm resonant conditions on a time scale of  $100\mu\text{s}$ . In the future further insight into the emission properties of single NVs could be obtained by interfering photons from a single emitter in an unbalanced interferometer [10].

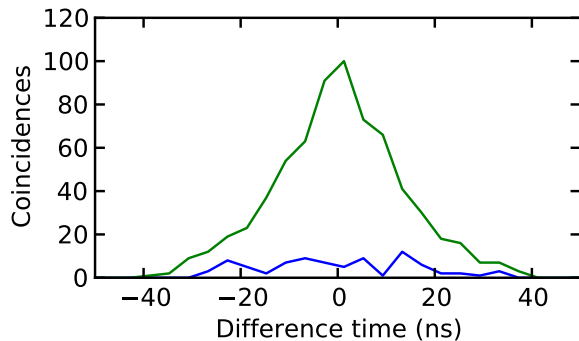

FIG. S6. Two-photon quantum interference between indistinguishable single photons leads to bunching at the output of a beam splitter. This is reflected in a suppressed probability of detecting coincident clicks at each APD during the same entanglement generation element (blue). This interference is not present for events in which one APD clicks during one entanglement generation element, while the other APD clicks during the next entanglement generation element (green).

## IX. PHASE STABILITY

As mentioned in Section VII B, in order to create the initial spin-photon entanglement, resonant laser pulses are used to selectively excite the  $|m_s = 0\rangle$  state to a higher level; this excited state then spontaneously decays, emitting a single photon. In this way, the photon-number occupation of the emission optical mode becomes entangled with the state of the NV. This resonant excitation process imprints the phase of the excitation laser onto the resulting spin-photon state. As the optical mode propagates towards the beam splitter, it also picks up an additional phase that depends on the optical path length that it traverses. After the optical modes from each NV interfere on the beam splitter and a photon is detected, the resulting spin-spin entangled state has a phase  $\phi$  that depends on the total phase difference between the two spin-photon states.

Since we derive the resonant excitation pulses from the same laser, the full setup effectively acts as an optical interferometer (Fig S7A), starting from where the excitation pulses are split, and ending at the beam splitter at which the photons are interfered. The phase sensitivity of

the resulting spin-spin entangled state is the same as for classical light traversing the same paths, but reflecting off of the NV sample instead of exciting the NV. By probing the stability of the interferometer using classical light, we can therefore determine the expected difference between  $\phi_1$  and  $\phi_2$  for subsequent entangled states. This allows us to determine how much the interferometer phase stability will impact the fidelity of the resulting purified state.

Fig. S7B shows measurements of the output intensity of one port of the beam splitter, measured using a photodiode. As the interferometer is not phase stabilized, the output fluctuates over time. The noise spectral density for this signal is shown in Fig. S7C. Several clear resonances can be seen below 1 kHz; these dominate the dynamics of the interferometer.

A useful measure for quantifying the phase stability of the interferometer is the standard deviation  $\Delta\phi$  of the phase difference  $\delta\phi(\tau) = \phi(t + \tau) - \phi(t)$  between two sample points separated by a fixed time difference  $\tau$ , measured for all  $t$  in the sample. This is plotted in Fig. S7D. As can be seen, the standard deviation  $\Delta\phi$  grows rapidly for the first millisecond, and then oscillates more slowly. These oscillations are caused by several resonant frequencies that dominate the noise spectrum of the interferometer, as is shown in Fig. S7C.

Once the first entangled state is created, the swap operations take 0.961 ms. For the data of Fig. S7, this would lead to an initial phase deviation of  $\Delta\phi \approx 0.18$  rad. Each entanglement generation attempt during the second stage takes  $7\mu\text{s}$ . We do not try more than 500 times to generate an entangled state the second time, and so the phase deviation would not increase beyond  $\Delta\phi \approx 0.24$  rad. Therefore, for the data in Fig. S7, we find an estimated dephasing probability of 0.018. Since the interferometer is not monitored during the experiment, these estimates can only serve as a guide. In our modeling we use the phase stability as a free parameter, fitting a linearly increasing phase deviation with  $\Delta\phi = 0.49$  rad after 1 ms, which is larger but of the same order as that measured in Fig. S7.

## X. EBIT RATE ESTIMATES

### A. Distillation

From our experimental data, we can determine the total number of successful events  $n_s$ , as well as the total number of entangling attempts made  $n_a$ . From these numbers and the duration of an entanglement attempt  $t_e = 7\mu\text{s}$ , we can estimate the instantaneous rate  $r = n_s/(n_a t_e)$  at which the protocol succeeds (i.e. the rate assuming that both NVs are on resonance, a condition which is necessary for any network protocol). As shown in Fig. S8A, this rate is a function of the superposition angle  $\theta$ .

The distillable entanglement of a state  $\rho$  is upper bounded by its logarithmic negativity  $E_N(\rho)$ , an easily

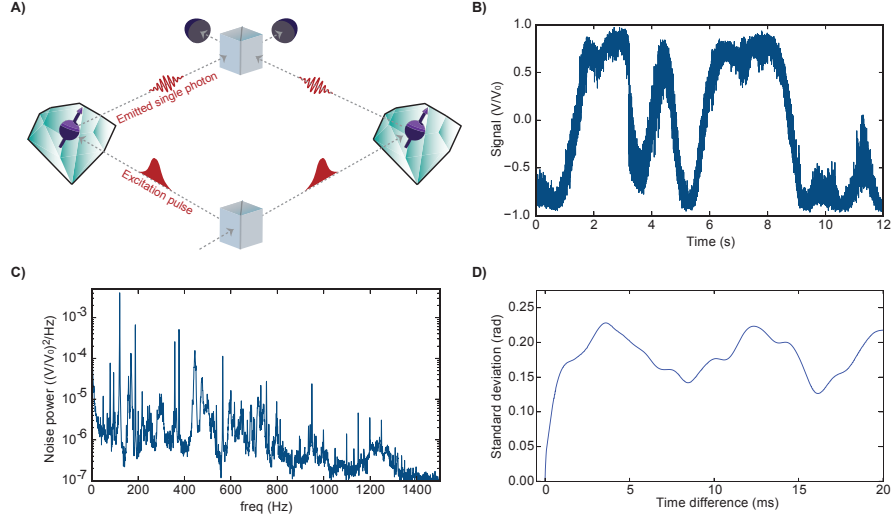

FIG. S7. a) The entanglement protocol imprints a phase on the entangled state that depends on the relative phase of the excitation laser pulses, as well as the difference in the phase acquired by the single photons as they propagate from the NVs to a central beam splitter. This creates an effective interferometer, starting where the excitation pulses are separated at an initial beam splitter, and ending at the final beam splitter. b) Classical light traversing the interferometer, but reflecting off of the NV sample instead of exciting the NV, is subject to the same phase fluctuations as the entangled states. This allows us to easily probe the expected phase stability of the protocol. Here classical light is inserted into the interferometer, and the output intensity is measured at one output port of the final beam splitter using a photodiode. Fluctuations in the output intensity over time are seen due to changes in the relative path length. c) Noise spectral density of the interferometer output showing many several sharp resonances below 1 kHz. d) Standard deviation of the inferred phase difference between sets of sample points separated by a fixed time difference. As can be seen, a phase difference is rapidly acquired within about 1 ms, but then the dynamics are dominated by a few resonant frequencies that periodically increase and then decrease the phase difference.

computable entanglement measure [11].  $E_N(\rho)$  is determined by the sum of the singular values of the partial transpose of  $\rho$ . We do not have access to the full density matrix  $\rho$  for all of the  $\theta$  values that we measure. However, we can make an estimate of  $E_N(\rho)$  by assuming that all off-diagonal elements of the density matrix are zero, apart from the coherence  $c$  between  $|01\rangle$  and  $|10\rangle$ . This assumption is supported by our measurements of the density matrix for  $\theta = \pi/6$  (shown in Fig. 4A of

the main text), in which other off-diagonal terms were indeed negligible. Under this assumption, it is possible to calculate  $E_N(\rho)$  using only our measurements of the correlations  $\langle \hat{X}\hat{X} \rangle$ ,  $\langle \hat{Y}\hat{Y} \rangle$  and  $\langle \hat{Z}\hat{Z} \rangle$ . Parameterizing  $\rho$  as

$$\begin{pmatrix} 1 - r - p_{11} & 0 & 0 & 0 \\ 0 & r - p_{10} & c & 0 \\ 0 & c^* & p_{10} & 0 \\ 0 & 0 & 0 & p_{11} \end{pmatrix}, \quad (7)$$

$$E_N(\rho) = \log_2 \left( r + \frac{1}{\sqrt{2}} (\sqrt{\alpha + (1-r)(1-r+\beta)} + \sqrt{\alpha + (1-r)(1-r-\beta)}) \right) \quad (8)$$

$$\begin{aligned} \text{where } \alpha &= 2|c|^2 + 2p_{11}^2 - 2p_{11}(1-r), \\ \beta &= \sqrt{4|c|^2 + (1-r-2p_{11})^2}. \end{aligned}$$

The logarithmic negativity is plotted in Fig. S8B for different values of  $\theta$ .

Multiplying the success rate by the distillable entanglement gives us the ebit rate. Since the number of ebits available depends on the number of second round en-

tanglement attempts needed to succeed, we carry out this calculation for different sets of our experimental results, binned by the number of second round attempts. We choose bins separated by fifty entangling attempts. This represents a compromise between having enough experimental results in each bin to calculate the correlations with reasonable accuracy, while not averaging too broadly over the different outcomes.

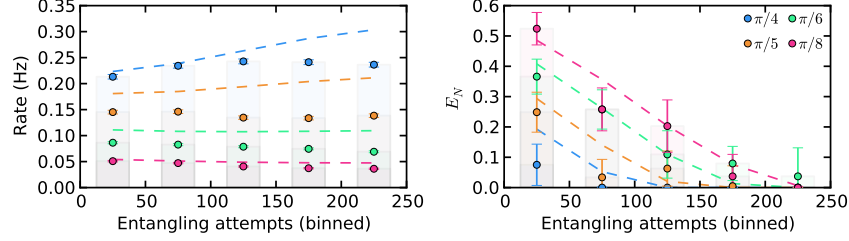

FIG. S8. a) The corresponding estimated protocol success rate (error bars are smaller than the points). Also shown in both plots are the predictions of our model (dashed lines). We partially attribute the deviation of the model to ionization of the NV electron spin while trying to generate entanglement. b) The experimentally estimated distillable entanglement  $E_N$  of the purified state as a function of  $\theta$  and elapsed second round entanglement generation attempts.

### B. Experimental model

Independent measurements allow us to estimate the probabilities of detecting a single photon given that one or other of the NVs was in the  $|0\rangle$  state (Table S2). From these probabilities, we can estimate the probability  $p_1$  of an entanglement generation attempt succeeding in the first round of the protocol. This in turn allows us to estimate  $p_2 = p_1(1 - p_1)^{n-1}$ , the probability of a second entanglement event occurring after a specified number of attempts  $n$ , given that the first round succeeded. In addition to these parameters, our model (Section VII) allows us to predict the probability of the local distillation gate succeeding, given the overall electron nuclear-spin state resulting from a specified number of second round entanglement generation attempts. Combining these numbers with the probability of a successful read-out after the distillation gate (0.9 on each side) gives us the average number of attempts (and therefore the time) necessary to produce a successful entanglement event. Our model also allows us to directly calculate  $E_N(\rho)$  from the simulated density matrix  $\rho$ . The rate and  $E_N$  predictions of our model are plotted alongside the experimental data in Fig. S8. This information is used to provide the theoretical lines in Fig. 5 of the main text.

### C. Comparison to Barrett and Kok protocol

The single-photon detection probabilities can also be used to estimate the rate that would be achieved for a conventional Barrett-Kok (BK) protocol [12] running on our experimental apparatus. Given these probabilities (Table S2), the BK success probability is given by  $\frac{1}{2}p_{d1}p_{d2}$ . As each entanglement attempts takes  $7\mu\text{s}$ , this gives a rate of 16 mHz.

In order to calculate the number of ebits available for the BK protocol, we assume that the generated state is perfect, apart from a reduced coherence  $c = V/2$  resulting from the imperfect indistinguishability  $V$  of our photons.

In this case

$$\begin{aligned} E_N(\rho) &= \log_2(1 + 2|c|) \\ &= \log_2(1 + V). \end{aligned} \quad (9)$$

The estimated rate and number of ebits are combined to give the BK ebit rates shown in Fig. 5 of the main text.

## XI. NUCLEAR INITIALIZATION AND READ-OUT SEQUENCES

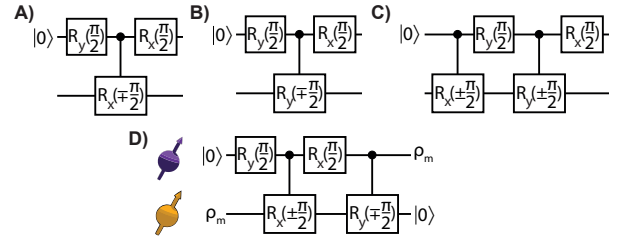

FIG. S9. Panels A-C) Read-out sequences of the nuclear spin expectation values  $\hat{X}$ ,  $\hat{Y}$ ,  $\hat{Z}$  [2]. All gate circuits are followed by a single-shot measurement of the electron spin. Panel D) Nuclear spin initialization sequence.  $\rho_m = \mathbb{I}/2$  is the mixed state.

Nuclear spins in each setup are initialized and read-out by employing conditional electron-nuclear gates and single-shot quantum measurements of the electron. Fig. S9 shows all relevant circuit diagrams for initialization and read-out of the nuclei. The directions of the rotations induced on the memory qubits by the controlled  $\pm\pi/2$  gates are determined by the communication qubit states.

Besides using established gate circuits for the tomography of single nuclear spins, we employ a sequential tomography for the combined electron-nuclear Bell states of Fig. 2 of the main text. Here, we first rotate the electron spin by applying one of six suitable microwave pulses

followed by a single-shot read-out measurement. We continue with the measurement tomography sequence of the nuclear spin if the electron was successfully measured to be in  $|m_s = 0\rangle$ . This guarantees a high projectivity and allows for the implementation of the nuclear-spin read-out sequence with high fidelity as the  $|m_s = 0\rangle$  minimally dephases the nuclear spin.

## XII. P-VALUES FOR DISTILLATION

As noted in the main text, successful distillation requires that the distilled state is increased in fidelity as compared to the raw states. In order to provide evidence that this is the case, we calculate P-values for the measured state fidelities shown in Fig. 4B of the main text (replotted in Fig. S10), taking as a null hypothesis that the states do not show an increase in fidelity from the highest fidelity raw state. These P-values are given in Table S3.

| $\sin^2(\theta)$ | P-value comm. qubit state | P-value phase-stable state |
|------------------|---------------------------|----------------------------|
| $\pi/8$          | 0.26                      | 0.41                       |
| $\pi/6$          | 0.26                      | 0.41                       |
| $\pi/5$          | 0.0095                    | 0.023                      |
| $\pi/4$          | 0.0032                    | 0.0086                     |

TABLE S3. P-values for the null hypothesis that the final state fidelity is not increased from the highest-fidelity raw state.

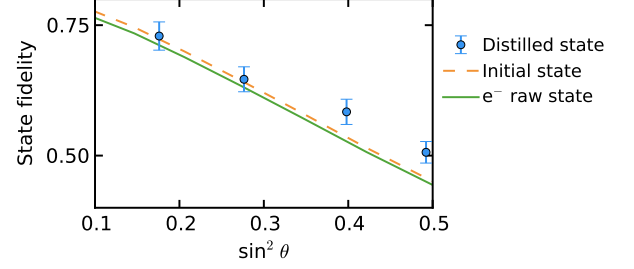

FIG. S10. Distilled state fidelities (blue) and communication qubit raw state fidelities (green) reproduced from Fig. 4B of the main text. Also shown is the best-case fidelity of the raw state if the optical phase was perfectly known at all points of the protocol (dashed orange).

Also calculated are the P-values showing evidence for distillation in the most stringent possible case, in which the raw states were generated in a completely stable interferometer with no phase drifts whatsoever (dashed orange line in Fig. S10). In this case the only imperfections on the raw states result from imperfect two-photon quantum interference, imbalanced optical losses, and dark counts. All of these quantities are independently characterized for our experiment.

## XIII. MEASURED DENSITY MATRICES

For completeness we present all numerical entries of all measured density matrices in this section. The matrices were directly reconstructed from the measurement outcomes via linear inversion. From Fig. 2B of the main text for node A:

$$\begin{pmatrix} 0.06(1) & 0.06(1) + i0.00(1) & 0.02(1) - i0.02(1) & 0.01(1) + i0.00(1) \\ 0.06(1) + i0.00(1) & 0.48(1) & -0.48(1) + i0.00(1) & -0.01(1) + i0.01(1) \\ 0.02(1) + i0.02(1) & -0.48(1) + i0.00(1) & 0.47(1) & -0.03(1) + i0.00(1) \\ 0.01(1) + i0.00(0) & -0.01(1) - i0.01(1) & -0.03(0) + i0.00(1) & -0.01(1) \end{pmatrix}. \quad (10)$$

and node B:

$$\begin{pmatrix} 0.00(1) & 0.01(1) + i0.02(1) & 0.00(1) - i0.02(1) & 0.00(1) + i0.01(1) \\ 0.01(1) - i0.02(1) & 0.51(1) & -0.49(1) - i0.02(1) & -0.01(1) + i0.03(1) \\ 0.00(1) + i0.02(1) & -0.49(1) + i0.02(1) & 0.47(1) & 0.00(1) - i0.02(1) \\ 0.00(1) - i0.01(1) & -0.01(1) - i0.03(1) & 0.00(1) + i0.02(1) & 0.02(1) \end{pmatrix}. \quad (11)$$

The density matrices of Fig. 4A of the main text are given in the following:

$$\begin{pmatrix} 0.11(2) & -0.01(3) + i0.02(3) & 0.03(3) + i0.01(3) & 0.00(3) - i0.02(4) \\ -0.01(3) - i0.02(3) & 0.43(2) & 0.20(3) + i0.03(4) & -0.04(3) - i0.03(3) \\ 0.03(3) - i0.01(3) & 0.20(3) - i0.03(4) & 0.46(2) & 0.07(3) - i0.05(3) \\ 0.00(3) + i0.02(4) & -0.04(3) + i0.03(3) & 0.07(3) + i0.05(3) & 0.00(2) \end{pmatrix} \quad (12)$$

$$\begin{pmatrix} 0.13(2) & 0.06(3) - i0.05(3) & 0.02(3) + i0.05(3) & 0.00(3) + i0.05(3) \\ 0.06(3) + i0.05(3) & 0.40(2) & -0.21(3) + i0.01(3) & -0.04(3) - i0.03(3) \\ 0.02(3) - i0.05(3) & -0.21(3) - i0.01(3) & 0.45(2) & 0.02(3) - i0.01(3) \\ 0.00(3) - i0.05(3) & -0.04(3) + i0.03(3) & 0.02(3) + i0.01(3) & 0.02(2) \end{pmatrix} \quad (13)$$

Numbers in brackets represent one standard deviation.

- 
- |                                                                                                                                                                                                                                                                                                                                                                                                                                                                                                                                                                         |                                                                                                                                                                                                                                                                                                                                                                                                                                                                                           |
|-------------------------------------------------------------------------------------------------------------------------------------------------------------------------------------------------------------------------------------------------------------------------------------------------------------------------------------------------------------------------------------------------------------------------------------------------------------------------------------------------------------------------------------------------------------------------|-------------------------------------------------------------------------------------------------------------------------------------------------------------------------------------------------------------------------------------------------------------------------------------------------------------------------------------------------------------------------------------------------------------------------------------------------------------------------------------------|
| <p>[1] B. Hensen, <i>et al.</i>, <i>Nature</i> <b>526</b>, 682 (2015).<br/> [2] J. Cramer, <i>et al.</i>, <i>Nat. Commun.</i> <b>7</b>, 11526 (2016).<br/> [3] N. Kalb, <i>et al.</i>, <i>Nat. Commun.</i> <b>7</b>, 13111 (2016).<br/> [4] L. Robledo, <i>et al.</i>, <i>Nature</i> <b>477</b>, 574 (2011).<br/> [5] A. Reiserer, <i>et al.</i>, <i>Phys. Rev. X</i> <b>6</b>, 021040 (2016).<br/> [6] E. T. Campbell, S. C. Benjamin, <i>Phys. Rev. Lett.</i> <b>101</b>, 130502 (2008).<br/> [7] N. H. Nickerson, J. F. Fitzsimons, S. C. Benjamin, <i>Phys.</i></p> | <p><i>Rev. X</i> <b>4</b>, 041041 (2014).<br/> [8] C. K. Hong, Z. Y. Ou, L. Mandel, <i>Phys. Rev. Lett.</i> <b>59</b>, 2044 (1987).<br/> [9] W. Pfaff, <i>et al.</i>, <i>Science</i> <b>345</b>, 532 (2014).<br/> [10] T. Legero, T. Wilk, M. Hennrich, G. Rempe, A. Kuhn, <i>Phys. Rev. Lett.</i> <b>93</b>, 070503 (2004).<br/> [11] M. B. Plenio, <i>Phys. Rev. Lett.</i> <b>95</b>, 090503 (2005).<br/> [12] S. D. Barrett, P. Kok, <i>Phys. Rev. A</i> <b>71</b>, 060310 (2005).</p> |
|-------------------------------------------------------------------------------------------------------------------------------------------------------------------------------------------------------------------------------------------------------------------------------------------------------------------------------------------------------------------------------------------------------------------------------------------------------------------------------------------------------------------------------------------------------------------------|-------------------------------------------------------------------------------------------------------------------------------------------------------------------------------------------------------------------------------------------------------------------------------------------------------------------------------------------------------------------------------------------------------------------------------------------------------------------------------------------|
